# Supplementary material for: Toward Pioneering Sensors and Features Using Large Language Models in Human Activity Recognition
Source: arXiv:2306.16017 source file (2023-06-28)
Supplement: Supplementary file 1 [file 9_appendix.tex]

\section*{Appendix}
\label{section:appendix}
